# Supplementary material for: Byzantine-Tolerant Methods for Distributed Variational Inequalities
Source: arXiv:2311.04611 source file (2023-11-08)
Supplement: Supplementary file 1 [file appendix.tex]

\appendix  %This command ends the counting of sections.
\tableofcontents
\input{appendix/auxilary}
\input{appendix/cc}
